# Supplementary material for: Electronic structure and topology across $T_c$ in magnetic Weyl semimetal Co$_3$Sn$_2$S$_2$
Source: arXiv:2105.08265 ancillary file (2021-10-21)
Supplement: Supplementary file 1 [file supp_for_v12.pdf]

# Supplementary Material: Electronic structure and topology across $T_c$ in magnetic Weyl semimetal $Co_3Sn_2S_2$

Antonio Rossi[1,2,*], Vsevolod Ivanov[2,*], Sudheer Sreedhar[2], Adam L. Gross[2], Zihao Shen[2], Eli Rotenberg[1], Aaron Bostwick[1], Chris Jozwiak[1], Valentin Taufour[2], Sergey Y. Savrasov[2], and Inna M. Vishik[2]

[1]Advanced Light Source, Lawrence Berkeley National Lab, Berkeley, 94720, USA
[2]Department of Physics and Astronomy, University of California, Davis, CA 95616, USA
[*]These two authors contributed equally

## Supplementary Note 1: Additional Details for Electronic Structure Simulations

Theoretical calculations were performed using two distinct methodologies. The electronic structure of $Co_3Sn_2S_2$ was computed with LmtART, using density functional theory and the full–potential linear–muffin–tin–oribtal method (FP-LMTO) with spin-orbit coupling [S1, S2], within the local density approximation (LDA) and local spin density approximation (LSDA). Subsequent calculations with the Hubbard correction (LDA+$U$), and disordered local moments (LDA+DLM) were also performed within this framework. LSDA and LDA+$U$ band structures computed with this way are shown below (Fig. S1).

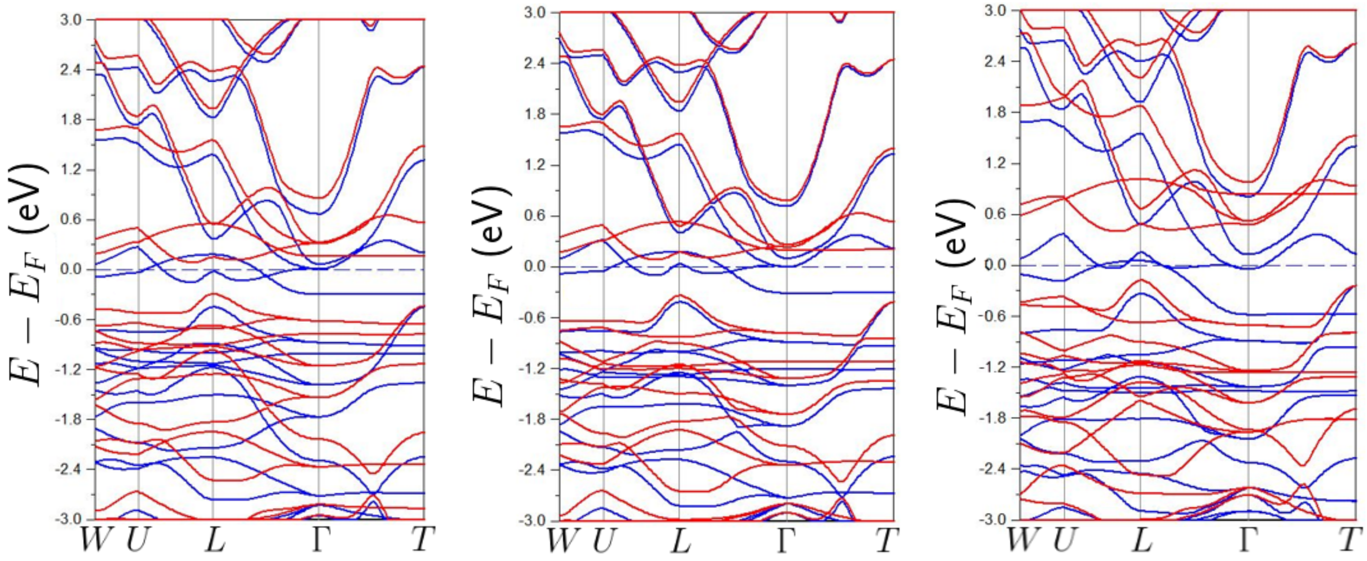


Figure S1: Band structures of $Co_3Sn_2S_2$ calculated with FP-LMTO, with spin up (blue) and spin down (red) bands indicated, computed using LSDA (left), LDA+$U$ = 2eV (middle), and LDA+$U$ = 4eV (right).

Additionally, first–principles simulations of $Co_3Sn_2S_2$ were performed using the Quantum ESPRESSO package [S3, S4]. These were also done within LDA and LSDA, using projector augmented waves (PAW) in the plane wave basis with spin-orbit coupling included. Exchange and corelation terms were included through the Perdew-Burke-Ernzerhof (PBE) parameterization scheme as implemented in pslibrary21 [S5]. Scalar relativistic PAW pseudopotentials were used. The experimental lattice constants [S6] were used in computing the electronic structures for the primitive unit cell (1X) on a $10 \times 10 \times 10$ $\boldsymbol{k}$-point grid, and for the hexagonal standard cell including three formula units (3X) on a $10 \times 10 \times 4$ $\boldsymbol{k}$-point grid. These calculations were then projected onto a basis of maximally localized Wannier functions using the WANNIER90 package [S7], with the following initial set of orbitals: Co-3$d$, Sn-5$sp$, and S-3$p$. The resulting band structure is plotted along $K - \Gamma - K$ (Figure S2).

The supercell Hamiltonian $\mathcal{H}_{ij}(\boldsymbol{R})$ was constructed in the following fashion. The original unit cell and associated realspace Hamiltonian in the Wannier basis $H(\boldsymbol{r})$ are stacked into a $N$-unit supercell in the $k_z$ direction, corresponding to [111] for the 1X and [001] for the 3X unit cells respectively. These stacked unit cells are indexed by $i$ and $j$, with the vectors $\boldsymbol{t}_i$ and $\boldsymbol{t}_j$ pointing to the associated unit cells. The hoppings of the supercell Hamiltonian are defined as follows:

$$\mathcal{H}_{ij}(\boldsymbol{R}) = \mathcal{H}_{ij}(\boldsymbol{r} + \boldsymbol{t}_i - \boldsymbol{t}_j) = H(\boldsymbol{r}). \tag{1}$$

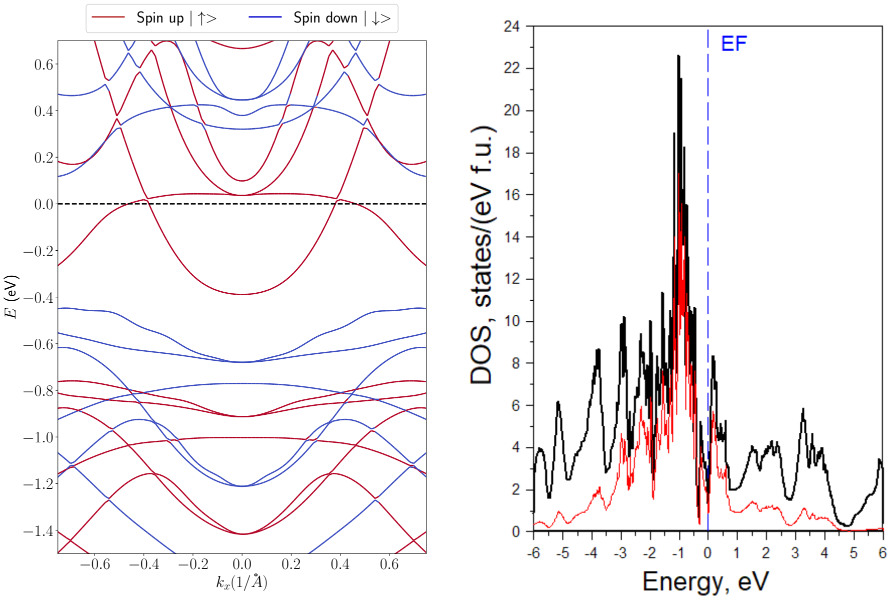


Figure S2: Left: Bulk band structure of $Co_3Sn_2S_2$ computed with LSDA and projected onto a basis of Wannier functions, with spin up (red), and spin down (blue) bands indicated. Right: Density of states, with Co-3$d$ contribution shown in red.

From there, the slab Hamiltonian can be obtained by setting all hoppings that cross the plane between the top unit cell $i = N$ and bottom unit cell $i = 1$ of the supercell above. We found that for the primitive unit cell layered in the $k_z$ direction, the uneven surface and hanging atoms at the termination, resulted in a number of parasitic surface states. The 3X unit cells reproduced all of the known surface states of $Co_3Sn_2S_2$, and so were used for all slab calculations and comparisons with experiment. The computed slab band structures along the $K - \Gamma - K$ direction of the two dimensional BZ are shown in Figure S3.

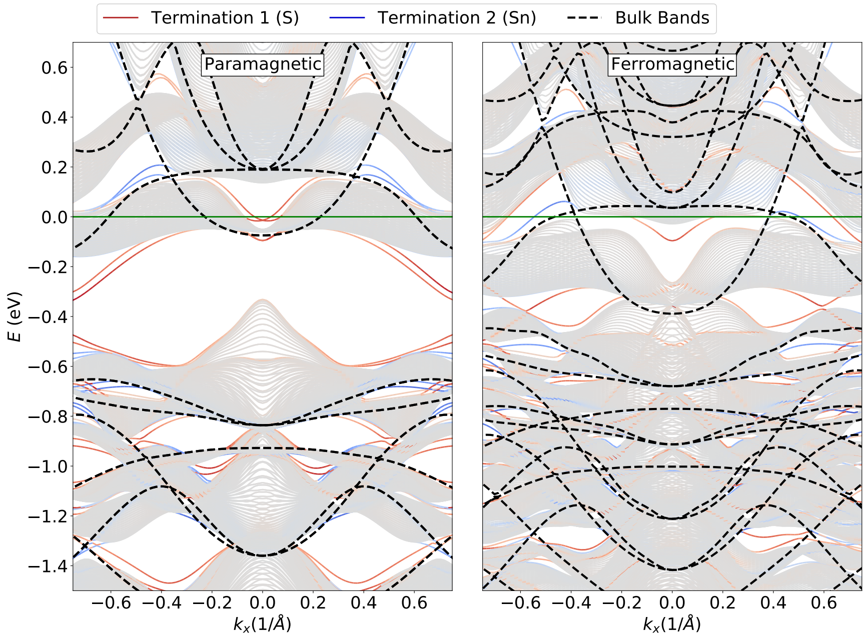


Figure S3: Computed band structure for a 60 formula unit slab Hamiltonian for non-magnetic (left) and ferromagnetic (right) LSDA. The single unit cell bulk band structures are plotted with a black dashed lines. The surface characters for the Sn-termination (blue), S-termination (red), and non-surface(grey).

We additionally compute the density of states (DOS) within LSDA (Figure S2) in order to estimate the electronic contribution to the heat capacity. There is a dip in the density of states near the Fermi energy due to the gap in spin down bands, which means only spin up bands contribute at those energies. We find that the density of states $N(E_f) = 1.377$ states/eV per formula unit (f.u.), which corresponds to a Sommerfield $\gamma_{\text{th}} = 3.25$ mJ mol$^{-1}$ K$^{-1}$.

## Supplementary Note 2: Derivation of Tight Binding Model

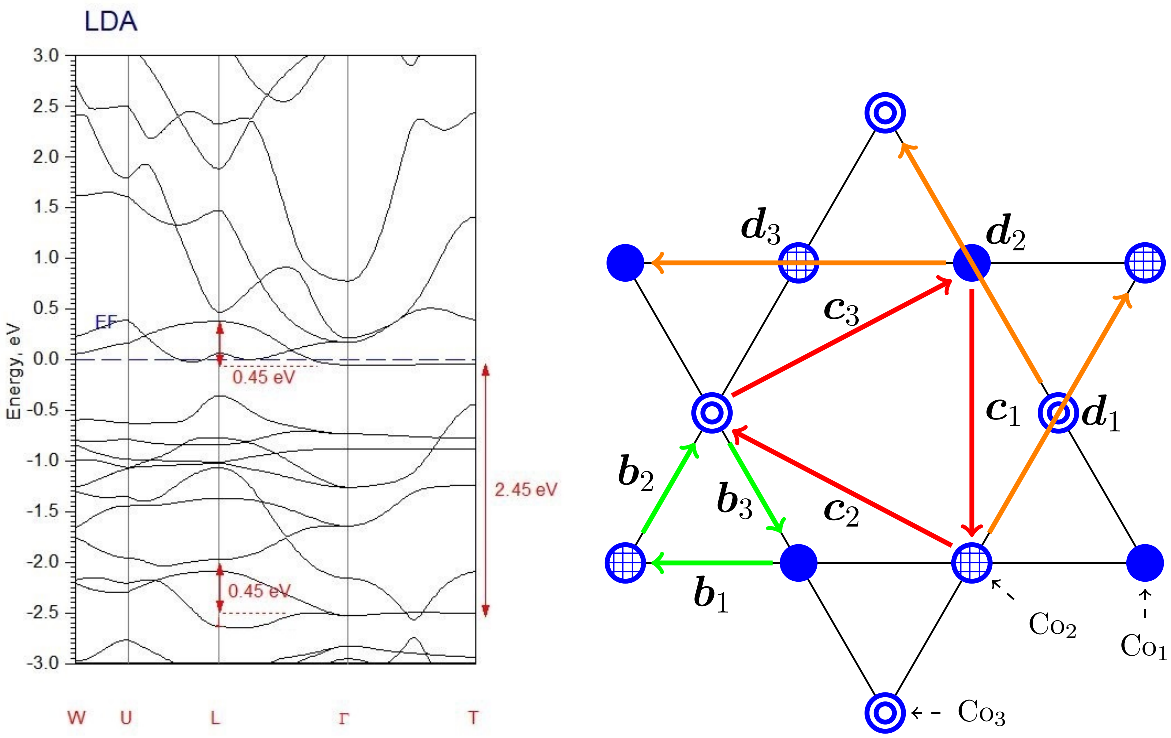


Figure S4: Left: Bandstructure of $Co_3Sn_2S_2$ computed within the spinless local density approximation. Right: Hopping vectors for the three–orbital in–plane tight–binding model on the kagome lattice. Nearest–neighbor $\boldsymbol{b}_i$ (green), next–nearest–neighbor $\boldsymbol{c}_i$ (red), and next–next–nearest–neighbor $\boldsymbol{d}_i$ (orange) vectors are shown.

Here we detail the extraction of tight–binding coefficients from the electronic structure calculation. We consider a tight–binding model of $d_{x^2-y^2}$ orbitals on the kagome lattice of Co atoms, with each orbital rotated to respect the local three–fold symmetry: $Co_1$ rotated by $+\pi/12$, $Co_2$ by $-\pi/12$ and $Co_3$ by $\pi/4$. With the orbitals rotated to respect the local symmetry, this model becomes equivalent to one with spherical $s$-orbitals on the kagome lattice.

The LDA calculation (Fig S4) shows that the $d_{x^2-y^2}$ band has almost no dispersion along the $k_z$ direction, meaning out of plane hoppings are negligible. Furthermore, the non-vanishing dispersion along the $k_x$-$k_y$ directions guarantees higher order in–plane hoppings beyond nearest–neighbor, which would result in an ideal flat band on the kagome lattice. In our model, we take into account the hoppings up to third order, as shown in Figure S4. For third–nearest–neighbor hoppings, we neglect the hopping that crosses the hexagonal face. Such a hopping would be mediated by exchange with the $p_z$ orbital of the Sn atoms that lie at the center of each hexagon, which we would expect to be small compared to hoppings along the Co atom lattice. For instance, for $Co_1$, we only include the hoppings along $\pm\boldsymbol{d}_2$ and $\pm\boldsymbol{d}_3$, neglecting those along $\pm\boldsymbol{d}_1$ which pass through the center of the hexagon.

The model Hamiltonian, $\mathcal{H}(\boldsymbol{k})$ can be written

$$\begin{aligned}\mathcal{H}(k) = \epsilon_d + 2t_1 \begin{pmatrix} 0 & \cos(\boldsymbol{k}\cdot\boldsymbol{b}_1) & \cos(\boldsymbol{k}\cdot\boldsymbol{b}_3) \\ \cos(\boldsymbol{k}\cdot\boldsymbol{b}_1) & 0 & \cos(\boldsymbol{k}\cdot\boldsymbol{b}_2) \\ \cos(\boldsymbol{k}\cdot\boldsymbol{b}_3) & \cos(\boldsymbol{k}\cdot\boldsymbol{b}_2) & 0 \end{pmatrix} + 2t_2 \begin{pmatrix} 0 & \cos(\boldsymbol{k}\cdot\boldsymbol{c}_1) & \cos(\boldsymbol{k}\cdot\boldsymbol{c}_3) \\ \cos(\boldsymbol{k}\cdot\boldsymbol{c}_1) & 0 & \cos(\boldsymbol{k}\cdot\boldsymbol{c}_2) \\ \cos(\boldsymbol{k}\cdot\boldsymbol{c}_3) & \cos(\boldsymbol{k}\cdot\boldsymbol{c}_2) & 0 \end{pmatrix} \\ + 2t_3 \begin{pmatrix} \cos(\boldsymbol{k}\cdot\boldsymbol{d}_2) + \cos(\boldsymbol{k}\cdot\boldsymbol{d}_3) & 0 & 0 \\ 0 & \cos(\boldsymbol{k}\cdot\boldsymbol{d}_1) + \cos(\boldsymbol{k}\cdot\boldsymbol{d}_3) & 0 \\ 0 & 0 & \cos(\boldsymbol{k}\cdot\boldsymbol{d}_1) + \cos(\boldsymbol{k}\cdot\boldsymbol{d}_2) & 0 \end{pmatrix},\end{aligned} \tag{2}$$

where $\epsilon_d$ is the onsite energy of the Co-3$d$ orbital, and $t_1$,$t_2$,$t_3$ are the hopping parameters. We can extract the values of these parameters by comparing with the LDA calculation for certain high symmetry points. At $\Gamma$, the eigenvalues are

$$\begin{aligned}\epsilon_1(\Gamma) &= \epsilon_d - 2t_1 - 2t_2 + 4t_3 \\ \epsilon_2(\Gamma) &= \epsilon_d - 2t_1 - 2t_2 + 4t_3 \\ \epsilon_3(\Gamma) &= \epsilon_d + 4t_1 + 4t_2 + 4t_3,\end{aligned} \tag{3}$$

while at the $L$ point, we find

$$\begin{aligned}\epsilon_1(L) &= \epsilon_d - 2t_1 + 2t_2 \\ \epsilon_2(L) &= \epsilon_d - 4t_3 \\ \epsilon_3(L) &= \epsilon_d + 2t_1 - 2t_2.\end{aligned} \tag{4}$$

Inspecting Figure S4, we can write down the following relationships between these energies:

$$\begin{aligned}\epsilon_3(\Gamma) - \epsilon_1(\Gamma) &= 6t_1 + 6t_2 = 2.46\text{eV} \\ \epsilon_3(L) - \epsilon_3(\Gamma) &= -2t_1 - 6t_2 - 4t_3 = 0.45\text{eV} \\ \epsilon_2(L) - \epsilon_2(\Gamma) &= 2t_1 + 2t_2 - 8t_3 = 0.45\text{eV},\end{aligned} \tag{5}$$

which can be solved to obtain the hopping parameters $t_1 = 0.77375\text{eV}$, $t_2 = -0.36375\text{eV}$, $t_3 = 0.04625\text{eV}$. Setting $\epsilon_d = -1.87\text{eV}$ correctly positions the bands with respect to $E_f$.

## Supplementary Note 3: Material Synthesis and Magnetic Characterization

The single crystals of $Co_3Sn_2S_2$ were synthesized by solution growth [S8, S9, S10]. A ternary mixture with initial composition $Co_{12}S_8Sn_{80}$ was first heated to 400 °C over two hours and held for another two hours. It was then heated to 1050 °C over six hours and held there for 10 hours, followed by slow cooling down to 740 °C within 90 hours. The remaining flux was removed by centrifugation. Shiny hexagonal crystals were obtained (Figure S5). The x-ray powder diffraction data refines to a hexagonal cell with $a = 5.3641(8)$Åand $c = 13.1724(9)$Åwhich are consistent with reported values [S11]. A field cooling curve with magnetic field of 1T parallel to $c$ axis is shown in Fig. S6, illustrating the ferromagnetic-paramagnetic transition. Fig. S7 shows the inverse susceptibility, with a Curie-Weiss fit revealing an effective moment of $0.98\mu_B$ per Co.

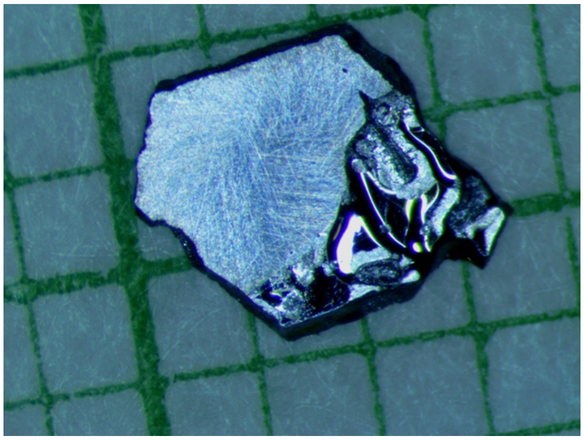

Figure S5: A crystal of $Co_3Sn_2S_2$.

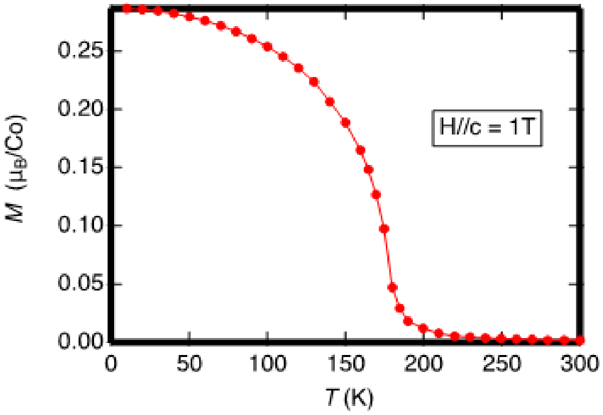


Figure S6: Temperature dependent magnetization under a magnetic field of 1T parallel to the c axis.

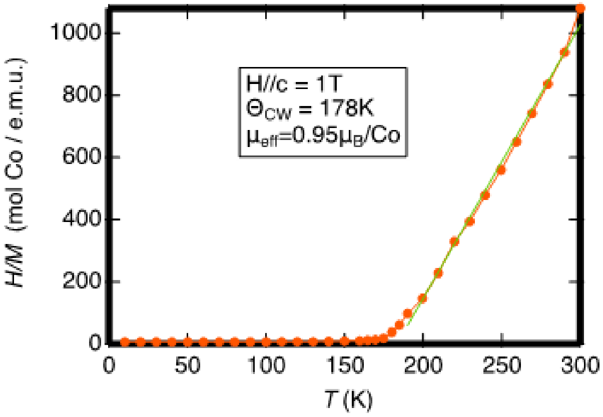


Figure S7: Temperature dependent inverse susceptibility of $Co_3Sn_2S_2$ with magnetic field parallel to the c axis.

## Supplementary Note 4: Additional ARPES data and comparisons to theory

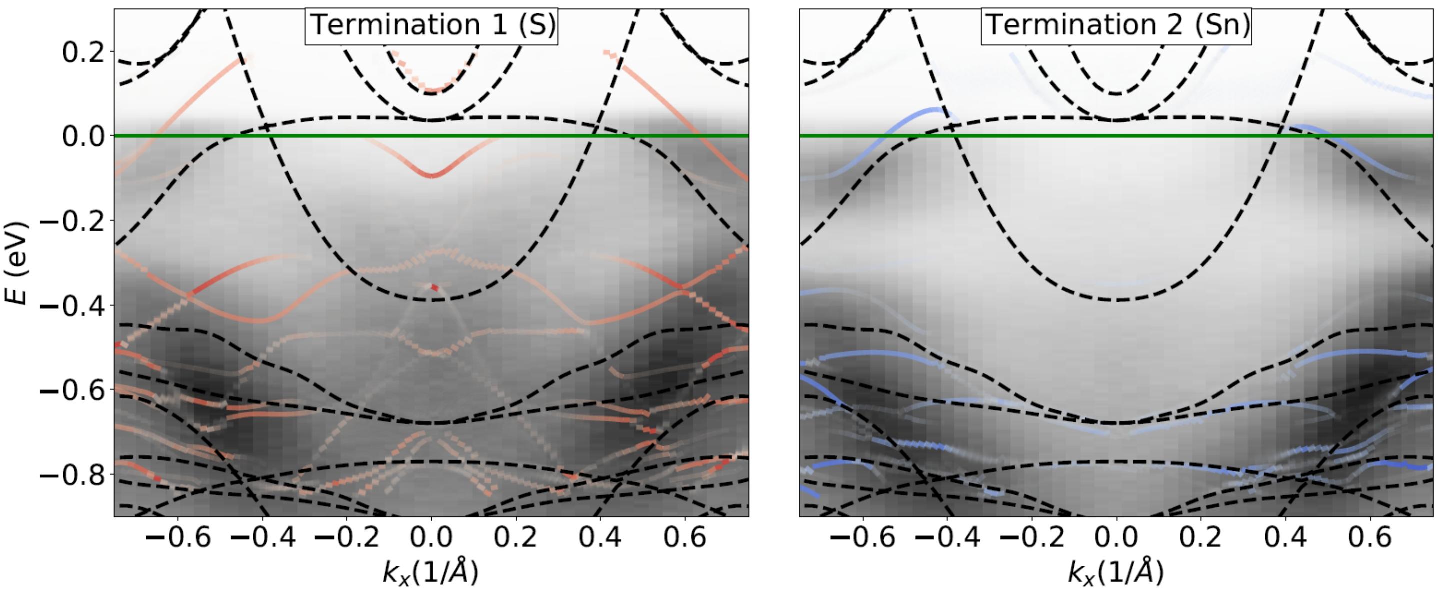


Figure S8: Slab calculations along the Γ-K cut for different surface terminations. Dashed lines indicate bulk bands, while slab bands are colored according to their character with red – S termination and blue Sn termination.

In Figure S8, we overlay the experimental $\Gamma - K$ cuts with surface state band structures obtained from theory calculations (Figure S8). These overlays indicate that the increased spectral density near Γ on the S termination can be well explained by the surface atomic orbital contributions for this termination. Furthermore, the S surface states near the $K$ point around $-0.3$eV may be a possible explanation for the apparent filled in spectral weight near this momentum, as compared to the open gap in the Sn termination. The apparent lack of Sn surface contribution near Γ further supports this assignment of the surfaces. It should be noted that the electronic structure methods we use may have an uncertainty on the order of $\sim$ 10meV in determining the Fermi energy, and the presence of electronic charges at the surface of the sample may further increase the energy discrepancy between measured and computed bands. Moreover, the pure S and Sn surface terminations being modeled here are a simplification which does not take nanoscale inhomogeneities into account. Nevertheless, the key qualitative spectral differences between the characteristic terminations are largely consistent with theory.

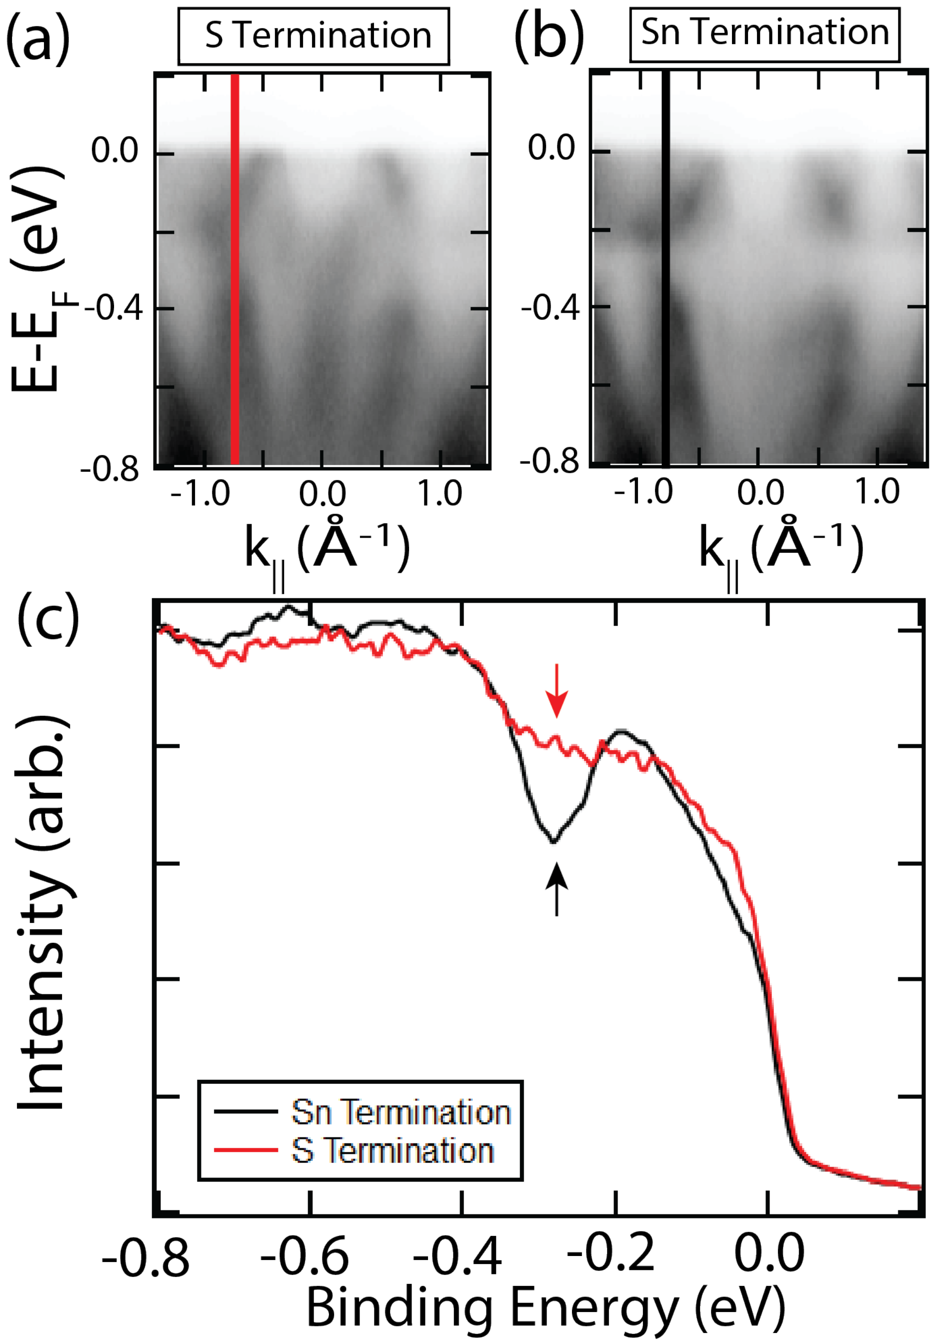


Figure S9: Termination-dependent EDCs, $T = 30$K. (a)-(b) Spectra along $\Gamma - K$ from main text, with vertical lines marking momenta where EDCs are compared. (c) EDCs on Sn and S terminations, with vertical arrows marking a gap in the former and filled-in spectral weight in the latter. EDC intensity normalized at $-0.8$eV.

In Figure S9 we compare EDCs near the K point to quantify differences in Sn and S termination spectra that may be difficult to discern in image plots. The Sn terminated spectra show a dip in spectral weight at $E \approx -0.3$eV, consistent with calculations in the main text and supplements (Fig. S3) which show a gap in that energy range. On the S termination, this dip is not nearly as pronounced, consistent with slab calculations that show S–derived surface states inside that gap.

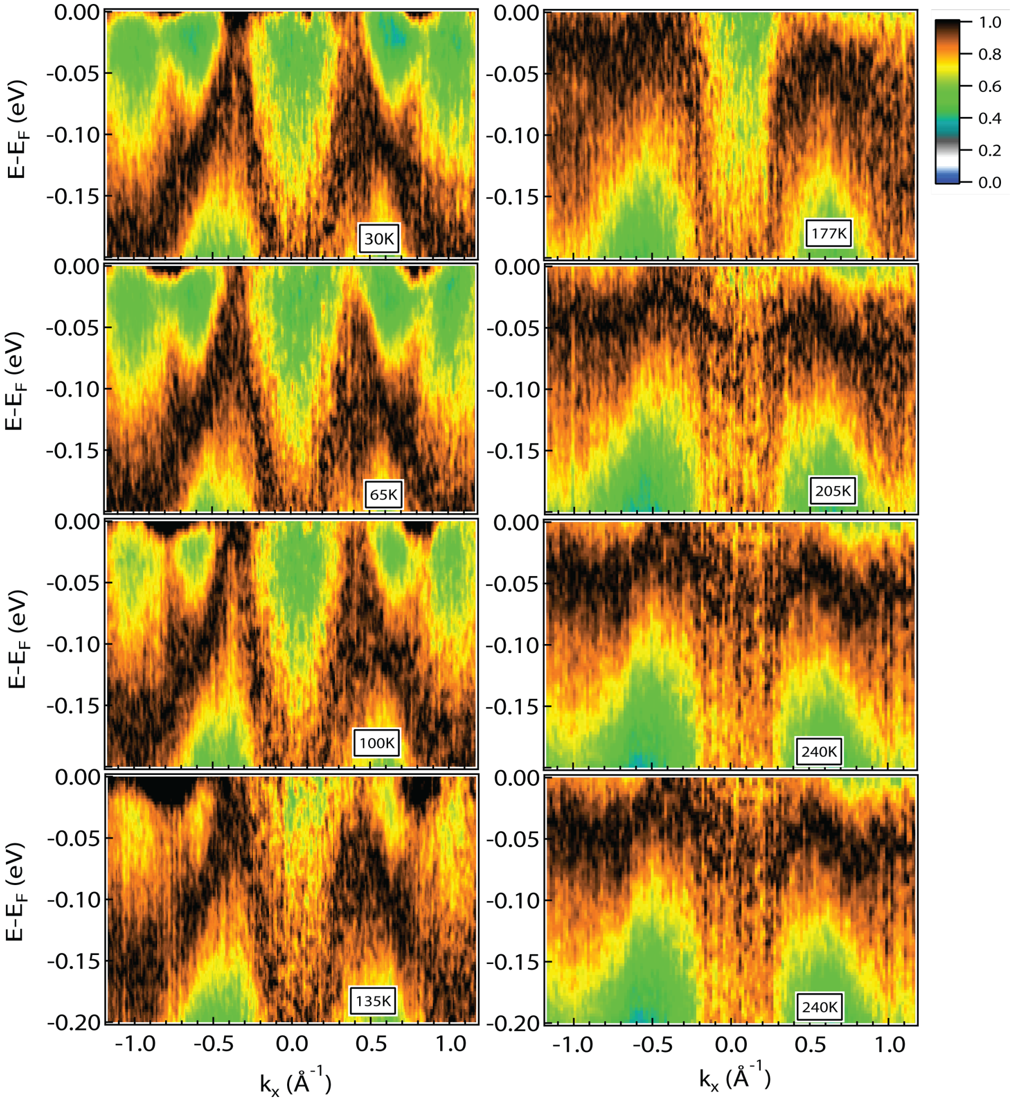


Figure S10: Temperature dependent cuts along M-K-Γ-K'-M cut trajectory, with every EDC in cut normalized to maximum. (a)-(d) Temperatures $\leq T_c$ (e)-(h) Temperatures $> T_c$

In Fig. S10, we show temperature-dependent high symmetry cuts from Fig. 6 of the main text (M-K-Γ-K'-M) plotted in a way that highlights weaker features near the Γ point. The plots in Fig. S10 normalize each EDC in the spectrum individually. Plotting the data in such a way highlights the dispersion of the EDC local maximum, and makes the band flattening across $T_c$ more visually apparent.

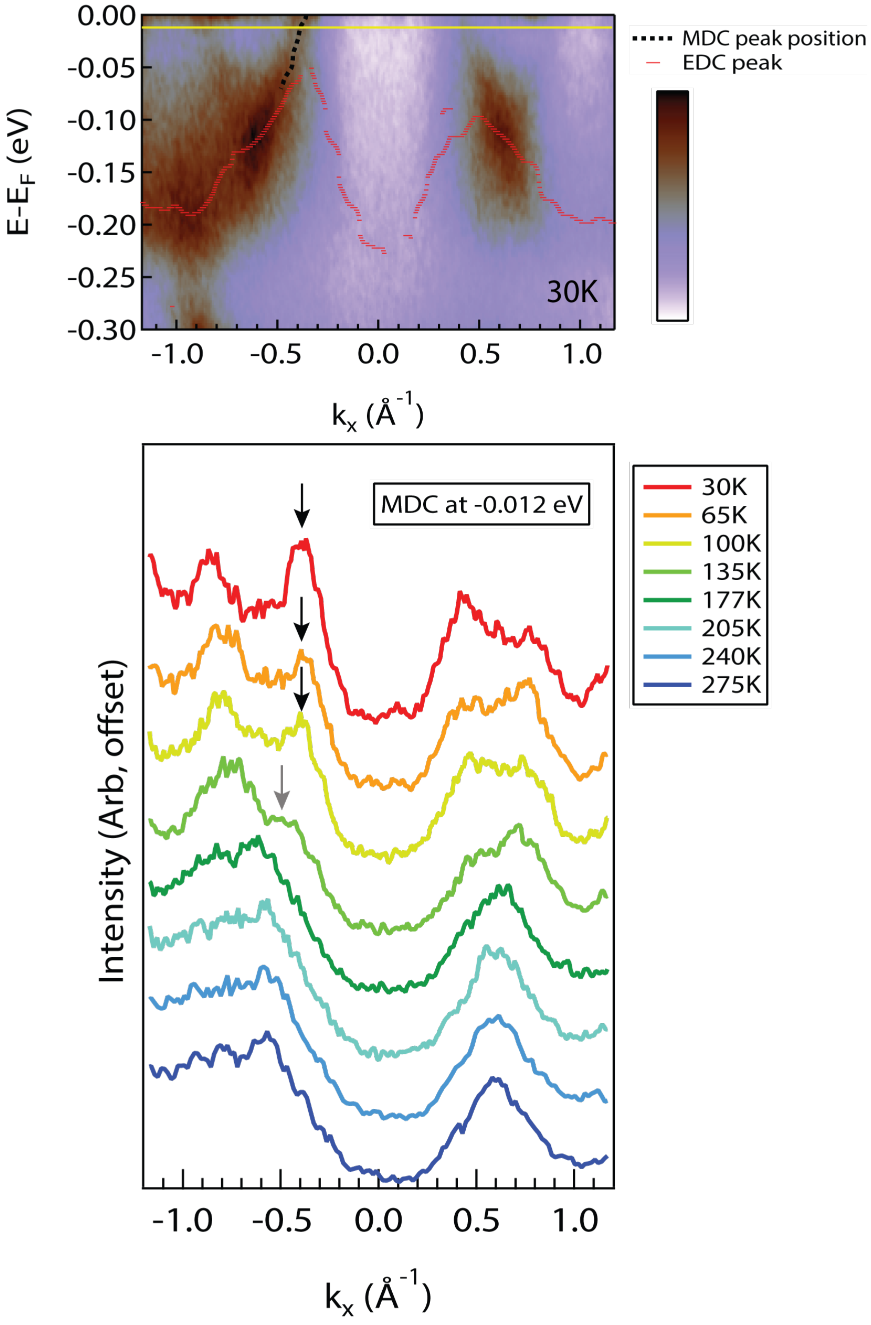


Figure S11: Temperature dependent MDCs through band which forms Fermi arc. (a) M-K-Γ-K'-M cut at 30K. Dotted line marks band which forms Fermi arc and red points mark EDC peak position. Yellow line marks energy where MDCs in panel (b) are taken. (b) MDCs at binding energy 12 meV. Arrows line peak originating from Fermi arc feature

Fig. S11 shows more raw data to demonstrate movement of Fermi arc approaching $T_c$. MDCs at $-12$ meV are shown, with this energy chosen because the band which forms the Fermi arc, as established by prior ARPES study [S12], is well separated from other spectral features. Arrows mark the peak in the MDC corresponding to the Fermi arc band. This feature does not disperse between 30K and 100K, and at 135K it is further from the Γ point. This feature is absent at $T_c$ =177K and higher temperatures.

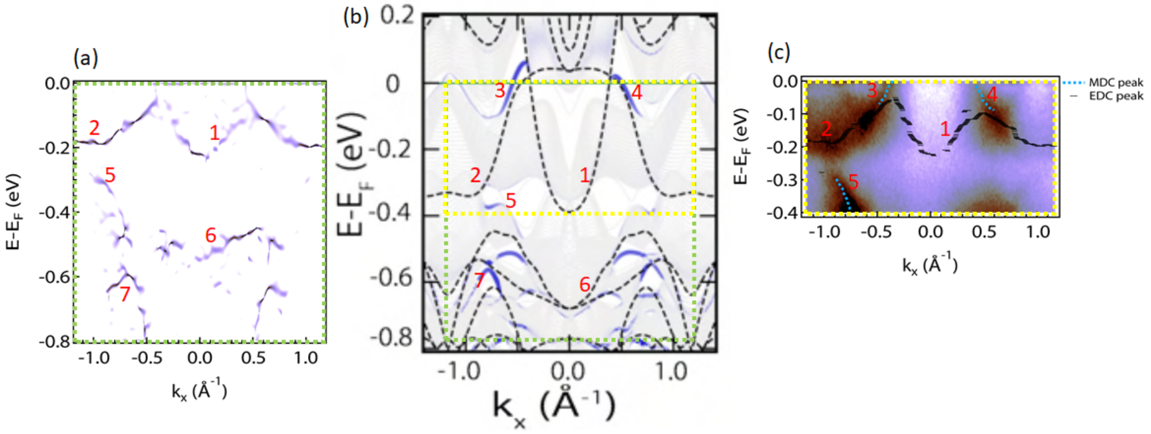


Figure S12: Correspondence between DFT calculations and ARPES spectral features on M-K-Γ-K'-M cut in the ferromagnetic state. (a) curvature plot to highlight higher energy features (b) Slab calculation for Sn termination from main text. Dashed lines indicate bulk bands. (c) Image plot to highlight low energy features, with dispersions derived from EDC local maxima and MDC peak fits marked. Labels 1-7 mark common features in theory and experiment. Green and yellow dashed boxes in (b) mark energy and momentum regions of panels (a) and (c)

Fig. S12 highlights the points of correspondence between theory and experiment, which are marked by numbers 1-7 in the figure. Features 1 and 2 mark the bulk bands that cross $E_F$. These have qualitative correspondence in theory and experiment, although the latter have a smaller bandwidth. Features 3 and 4 mark two surface bands characteristic of the Sn termination, with the former forming the Fermi arc connecting surface projections of Weyl points. Their inequivalency is discussed in the main text. There is again qualitative correspondence between theory and experiment. Feature 5 is another surface state located in the gap below the Fermi-crossing bulk bands, and a corresponding feature is present in the ARPES data. At higher binding energy, there are many bulk bands which are not all resolved in the ARPES experiment, likely because spectral broadening is comparable to the energy separation of different features. Nevertheless, electron-like bands near Γ (feature 6) is commonly present in both theory and experiment, as well as hole-like bands near K and K' (feature 7).

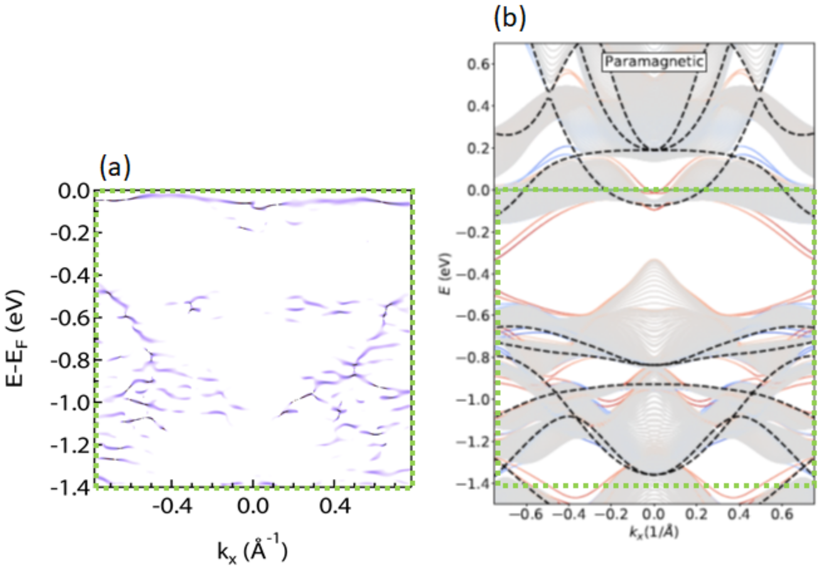


Figure S13: Comparison between computed band structure and ARPES spectral features on K-Γ-K'cut. (a) curvature plot at 205K (b) Computed band structure for a 60 formula unit slab Hamiltonian without magnetism (Fig. S3).

Fig. S13 compares spinless slab calculations from Fig. S3 to ARPES data at 205K, T>T$_c$. Although there are qualitative points of agreement between theory and experiment, with every experimental feature having a corresponding band in the calculation, the quantitative agreement is somewhat poorer than for the FM state. This reflects the increased importance of correlations above T$_c$, which are not captured in the model of Fig. S13(b). This indicates the in-adequateness of modeling the regime above T$_c$ with a total loss of local moments.

# References


[S1] S. Yu. Savrasov and D. Yu. Savrasov. Full-potential linear-muffin-tin-orbital method for calculating total energies and forces. *Phys. Rev. B*, 46:12181–12195, Nov 1992. doi: 10.1103/PhysRevB.46.12181. URL https://link.aps.org/doi/10.1103/PhysRevB.46.12181.

[S2] S. Y. Savrasov. Linear-response theory and lattice dynamics: A muffin-tin-orbital approach. *Phys. Rev. B*, 54:16470–16486, Dec 1996. doi: 10.1103/PhysRevB.54.16470. URL https://link.aps.org/doi/10.1103/PhysRevB.54.16470.

[S3] P Giannozzi, O Andreussi, T Brumme, O Bunau, M Buongiorno Nardelli, M Calandra, R Car, C Cavazzoni, D Ceresoli, M Cococcioni, N Colonna, I Carnimeo, A Dal Corso, S de Gironcoli, P Delugas, R A DiStasio, A Ferretti, A Floris, G Fratesi, G Fugallo, R Gebauer, U Gerstmann, F Giustino, T Gorni, J Jia, M Kawamura, H-Y Ko, A Kokalj, E Küçükbenli, M Lazzeri, M Marsili, N Marzari, F Mauri, N L Nguyen, H-V Nguyen, A Otero de-la Roza, L Paulatto, S Poncé, D Rocca, R Sabatini, B Santra, M Schlipf, A P Seitsonen, A Smogunov, I Timrov, T Thonhauser, P Umari, N Vast, X Wu, and S Baroni. Advanced capabilities for materials modelling with quantum ESPRESSO. *Journal of Physics: Condensed Matter*, 29(46):465901, oct 2017. doi: 10.1088/1361-648x/aa8f79. URL https://doi.org/10.1088/1361-648x/aa8f79.

[S4] Paolo Giannozzi, Stefano Baroni, Nicola Bonini, Matteo Calandra, Roberto Car, Carlo Cavazzoni, Davide Ceresoli, Guido L Chiarotti, Matteo Cococcioni, Ismaila Dabo, Andrea Dal Corso, Stefano de Gironcoli, Stefano Fabris, Guido Fratesi, Ralph Gebauer, Uwe Gerstmann, Christos Gougoussis, Anton Kokalj, Michele Lazzeri, Layla Martin-Samos, Nicola Marzari, Francesco Mauri, Riccardo Mazzarello, Stefano Paolini, Alfredo Pasquarello, Lorenzo Paulatto, Carlo Sbraccia, Sandro Scandolo, Gabriele Sclauzero, Ari P Seitsonen, Alexander Smogunov, Paolo Umari, and Renata M Wentzcovitch. QUANTUM ESPRESSO: a modular and open-source software project for quantum simulations of materials. *Journal of Physics: Condensed Matter*, 21(39):395502, sep 2009. doi: 10.1088/0953-8984/21/39/395502. URL https://doi.org/10.1088/0953-8984/21/39/395502.

[S5] Andrea Dal Corso. Pseudopotentials periodic table: From H to Pu. *Computational Materials Science*, 95:337–350, 2014. ISSN 0927-0256. doi: https://doi.org/10.1016/j.commatsci.2014.07.043. URL https://www.sciencedirect.com/science/article/pii/S0927025614005187.

[S6] Paz Vaqueiro and Gerard G. Sobany. A powder neutron diffraction study of the metallic ferromagnet Co3Sn2S2. *Solid State Sciences*, 11(2):513–518, February 2009. doi: 10.1016/j.solidstatesciences.2008.06.017. URL https://doi.org/10.1016/j.solidstatesciences.2008.06.017.

[S7] Arash A. Mostofi, Jonathan R. Yates, Young-Su Lee, Ivo Souza, David Vanderbilt, and Nicola Marzari. wannier90: A tool for obtaining maximally-localised Wannier functions. *Computer Physics Communications*, 178(9):685–699, 2008. ISSN 0010-4655. doi: https://doi.org/10.1016/j.cpc.2007.11.016. URL https://www.sciencedirect.com/science/article/pii/S0010465507004936.

[S8] Xiao Lin, Sergey L. Bud'ko, and Paul C. Canfield. Development of viable solutions for the synthesis of sulfur bearing single crystals. *Philosophical Magazine*, 92(19-21):2436–2447, 2012. doi: 10.1080/14786435.2012.671552. URL https://doi.org/10.1080/14786435.2012.671552.

[S9] Mohamed A. Kassem, Yoshikazu Tabata, Takeshi Waki, and Hiroyuki Nakamura. Single crystal growth and characterization of kagomé-lattice shandites Co3Sn2-xInxS2. *Journal of Crystal Growth*, 426:208–213, 2015. ISSN 0022-0248. doi: https://doi.org/10.1016/j.jcrysgro.2015.06.017. URL https://www.sciencedirect.com/science/article/pii/S0022024815004509.

[S10] V Nagpal and S Patnaik. Breakdown of Ohm's law and nontrivial Berry phase in magnetic Weyl semimetal Co3Sn2S2. *Journal of Physics: Condensed Matter*, 32(40):405602, jul 2020. doi: 10.1088/1361-648x/ab9859. URL https://doi.org/10.1088/1361-648x/ab9859.

[S11] S. Natarajan, G.V.Subba Rao, R. Baskaran, and T.S. Radhakrishnan. Synthesis and electrical properties of shandite-parkerite phases, A2M3Ch2. *Journal of the Less Common Metals*, 138(2):215–224, March 1988. doi: 10.1016/0022-5088(88)90110-5. URL https://doi.org/10.1016/0022-5088(88)90110-5.

[S12] D. F. Liu, A. J. Liang, E. K. Liu, Q. N. Xu, Y. W. Li, C. Chen, D. Pei, W. J. Shi, S. K. Mo, P. Dudin, T. Kim, C. Cacho, G. Li, Y. Sun, L. X. Yang, Z. K. Liu, S. S. P. Parkin, C. Felser, and Y. L. Chen. Magnetic Weyl semimetal phase in a Kagomé crystal. *Science*, 365(6459):1282–1285, September 2019. ISSN 0036-8075, 1095-9203. doi: 10.1126/science.aav2873. URL https://science.sciencemag.org/content/365/6459/1282. Publisher: American Association for the Advancement of Science Section: Report.
